# Supplementary material for: Robust Multivariate Estimation Based On Statistical Depth Filters
Source: arXiv:1909.04325 source file (2021-01-16)
Supplement: Supplementary file 1 [file depth-supplemental.pdf]

# Supplementary Material for "Robust multivariate estimation based on statistical data depth filters"

Giovanni Saraceno[1] and Claudio Agostinelli[1]

[1]Department of Mathematics, University of Trento, Trento, Italy, email: giovanni.saraceno@unitn.it

## Supplementary Material

Section SM–1 discusses the general properties that a statistical data depth function should satisfy. The derivation of the claim in Remark 1 is provided in Section SM–2.In Section SM–3, we prove that the general properties introduced in SM–1 hold for the Gervini-Yohai depth. Section SM–4 illustrates the univariate HS-filter with two-tails control and Section SM–5 contains full results of the Monte Carlo experiment. Finally, Section SM–6 reports the codes used for the multivariate Skew-Normal distribution example and for the Small-cap Stock Returns data set.

## SM–1 Statistical data depth properties

**Definition 1** (Depth Function)**.** *A* ***depth function*** $d(\cdot; F)$ *measures the centrality of a point w.r.t. a probability distribution* $F$.

$$d = \mathbb{R}^p \to \mathbb{R}^+ \cup \{0\}, \qquad \boldsymbol{x} \to d(\boldsymbol{x}; F)$$

A statistical depth function should satisfy the following Properties Liu [1990], Zuo and Serfling [2000]

**P1** Affine invariance: $d(\boldsymbol{x}; F) = d(\boldsymbol{A}\boldsymbol{x} + \boldsymbol{b}; F_{\boldsymbol{A},\boldsymbol{b}})$;

**P2** Maximality at center: if $F$ is "symmetric" around $\boldsymbol{\mu}$ then $d(\boldsymbol{x}; F) \leq d(\boldsymbol{\mu}; F)$ for all $\boldsymbol{x}$; for a more detailed discussion on symmetry see Serfling [2006].

**P3** Monotonicity: if (P2) holds, then

$$d(\boldsymbol{x}; F) \leq d(\boldsymbol{\mu} + \alpha(\boldsymbol{x} - \boldsymbol{\mu}); F) \qquad \alpha \in [0, 1] \ ;$$

**P4** Approaching zero: $\| \boldsymbol{x} \| \to \infty \Rightarrow d(\boldsymbol{x}; F) \to 0$.

# SM–2 Remark 1

Constructing our filter based on statistical depth functions, we divide $d_n$ by $2m$, where $m$ indicates the maximum value of the considered depth function, such that the maximum fraction of flagged outliers cannot exceed $\frac{1}{2}$. We wondered if the other filters have this property. Indeed, the filter firstly introduced by Gervini and Yohai [2002] has a similar characteristic.

Let $\boldsymbol{X} = X_1, \ldots, X_n$ be a random sample of observations and let $T_{0n}$ and $S_{0n}$ the initial location and dispersion estimators. Denote by $Z_i = \frac{X_i - T_{0n}}{S_{0n}}$ the standardized sample. Consider the chosen reference distribution $Z_i \sim F$. Indicating by $F^+$ the distribution of the absolute values of $Z_i$, denoted by $Y_i = |Z_i|$, and let $F_n^+$ be the empirical distribution. The proportion of detected outliers was defined as

$$d_n = \sup_{t \geq \eta} \{F^+(t) - F_n^+(t)\}^+,$$

where $\eta = (F^+)^{-1}(\alpha)$ is a large quantile of $F^+$ and $\alpha$ is a high order probability.

If $d_n \geq \frac{1}{2}$, then $\exists \ t^* \geq \eta$ such that

$$\begin{aligned} \frac{1}{2} \leq d_n &= F^+(t^*) - F_n^+(t^*) \\ &\leq 1 - F_n^+(t^*). \end{aligned}$$

Then, $F_n^+(t^*) \leq \frac{1}{2}$. This means

$$\begin{aligned} &\eta \leq t^* \leq median(\boldsymbol{Y}) \\ &\eta \leq median(\boldsymbol{Y}), \end{aligned}$$

where $\boldsymbol{Y} = (Y_1, \ldots, Y_n)$.

Consider now the order statistics $Y_{(i)} = |Z_{(i)}|$. We are interested in computing the probability that the median of $\boldsymbol{Y}$, denoted by $Y_{(\bar{n})}$, is greater then $\eta$. Note that, the value $\bar{n}$ depends if $n$ is odd or even, but it is not relevant

here. Considering the distribution function of order statistics we get

$$\begin{aligned}\mathbb{P}(Y_{(\bar{n})} > \eta) =& 1 - \mathbb{P}(Y_{(\bar{n})} \leq \eta) \\ =& 1 - \sum_{j=\bar{n}}^{n} \binom{n}{j} \left[F^{+}(\eta)\right]^{j} \left[1 - F^{+}(\eta)\right]^{n-j} \\ =& 1 - \sum_{j=\bar{n}}^{n} \binom{n}{j} \alpha^{j} (1-\alpha)^{n-j}.\end{aligned}$$

This quantity goes to 0 as $n \to \infty$. Note that, this is very small also for small values of $n$. To give an idea, for $n = 5$ and $\alpha = 0.95$, $\mathbb{P}(Y_{(\bar{n})} > \eta) = 0.0011$.

# SM–3 Gervini-Yohai depth

Here, we show that the Gervini-Yohai depth, defined as $d_{GY}(\boldsymbol{t}, F, G) = 1 - G(\Delta(\boldsymbol{t}, \boldsymbol{\mu}(F), \boldsymbol{\Sigma}(F)))$, is a proper statistical depth function, i.e., it satisfies the four properties introduced above.

1. Affine invariance: it follows directly from the affine invariance property of the Mahalanobis distance;

2. Maximality at center: if $F$ is elliptically symmetric around $\boldsymbol{\mu}(F)$,

   $$d_{GY}(\boldsymbol{\mu}(F), F, G) = 1 - G(\Delta(\boldsymbol{\mu}(F), \boldsymbol{\mu}(F), \boldsymbol{\Sigma}(F))) = 1 - G(0).$$

   For any $\boldsymbol{t} \neq \boldsymbol{\mu}(F)$ we have

   $$\begin{aligned}\Delta(\boldsymbol{t}, \boldsymbol{\mu}(F), \boldsymbol{\Sigma}(F)) &> 0 \\ G(\Delta(\boldsymbol{t}, \boldsymbol{\mu}(F), \boldsymbol{\Sigma}(F))) &\geq G(0) \\ 1 - G(\Delta(\boldsymbol{t}, \boldsymbol{\mu}(F), \boldsymbol{\Sigma}(F))) &\leq 1 - G(0) \\ d_{GY}(\boldsymbol{t}, F, G) &\leq d_{GY}(\boldsymbol{\mu}(F), F, G),\end{aligned}$$

   when $G$ is strictly monotone then strict inequality holds, and $\boldsymbol{\mu}(F)$ is the unique maximizer of the Gervini-Yohai depth.

3. Monotonicity:

   $$\begin{aligned}\Delta(\boldsymbol{\mu}(F) + \alpha(\boldsymbol{t} - \boldsymbol{\mu}(F)), \boldsymbol{\mu}(F), \boldsymbol{\Sigma}(F)) =& \\ &= (\alpha(\boldsymbol{t} - \boldsymbol{\mu}(F)))^{\top} \boldsymbol{\Sigma}(F)^{-1} (\alpha(\boldsymbol{t} - \boldsymbol{\mu}(F))) \\ &= \alpha^2 (\boldsymbol{t} - \boldsymbol{\mu}(F))^{\top} \boldsymbol{\Sigma}(F)^{-1} (\boldsymbol{t} - \boldsymbol{\mu}(F)) \\ &= \alpha^2 \Delta(\boldsymbol{t}, \boldsymbol{\mu}(F), \boldsymbol{\Sigma}(F)) \\ &\leq \Delta(\boldsymbol{t}, \boldsymbol{\mu}(F), \boldsymbol{\Sigma}(F))\end{aligned}$$

   Then $d_{GY}(\boldsymbol{\mu}(F) + \alpha(\boldsymbol{t} - \boldsymbol{\mu}(F)), F, G) \geq d_{GY}(\boldsymbol{t}, F, G)$.

4. Approaching zero: if $\| \boldsymbol{t} \| \to \infty$ we have that $\Delta(\boldsymbol{t}, \boldsymbol{\mu}(F), \boldsymbol{\Sigma}(F)) \to \infty$ and consequently $G(\Delta(\boldsymbol{t}, \boldsymbol{\mu}(F), \boldsymbol{\Sigma}(F))) \to 1$. Then

$$d_{GY}(\boldsymbol{t}, F, G) = 1 - G(\Delta(\boldsymbol{t}, \boldsymbol{\mu}(F), \boldsymbol{\Sigma}(F))) \to 0$$

# SM–4 Univariate filter with two-tails control

In the univariate case, given a point $x$, there exist only two half-spaces including it, hence, the half-space depth assumes the explicit form

$$\begin{aligned} d_{HS}(x; F) &= \min(P_F((-\infty, x]), P_F([x, \infty))) \\ &= \min(F(x), 1 - F(x) + P_F(X = x)). \end{aligned} \tag{1}$$

Let $X_1, \dots, X_n$ be an identically distributed sample, $X_i \in \mathbb{R}$ and consider the empirical distribution function $\hat{F}_n(\cdot)$. The sample halfspace depth will be

$$d_{HS}(x, \hat{F}_n) = \min\left(\frac{1}{n}\sum_{i=1}^{n} I(X_i \le x), \frac{1}{n}\sum_{i=1}^{n} I(X_i \ge x)\right). \tag{2}$$

Let $T_{0n}$ and $S_{0n}$ be a pair of initial location and dispersion estimators. Here, for $T_{0n}$ and $S_{0n}$, we choose the median and the median absolute deviation (MAD), respectively. For each observation $X_j$, we denote its standardized version by $Z_j = \frac{X_j - T_{0n}}{S_{0n}}$. Let $F$ be a chosen reference distribution for $Z = (Z_1, \dots, Z_n)$; here we use the standard normal distribution, i.e., $F = \Phi$. Let $\hat{F}_n$ be the empirical distribution for the standardized values, that is

$$\hat{F}_n(t) = \frac{1}{n}\sum_{i=1}^{n} I(Z_i \le t).$$

The proportion of flagged outliers can be expressed as

$$d_n = \max\left(\sup_{t \le -\eta_\beta} \{d_{HS}(t, \hat{F}_n) - d_{HS}(t, F)\}^+ ; \sup_{t \ge \eta_\beta} \{d_{HS}(t, \hat{F}_n) - d_{HS}(t, F)\}^+\right),$$

where $\eta_\beta = F^{-1}(\beta)$ is a large quantile of $F_j$. Note that, according to the general definition given in equation (1), the set $C^\beta(F) = \{x \in \mathbb{R} : d_{HS}(x, F) < d_{HS}(\eta_\beta)\}$ results in the simpler form written above considering the definition of the half-space depth in the univariate case. Now, consider the order statistics $Z_{(i)}$, and define $i_- = \min\{i : Z_{(i)} > -\eta_\beta\}$ and $i_+ = \max\{i : Z_{(i)} < \eta_\beta\}$. Using equations (1) and (2), the previous expression can be written as

$$d_n = \max\left(\sup_{i < i_-} \left\{\frac{i}{n} - F(Z_{(i)})\right\}^+, \sup_{i > i_+} \left\{F(Z_{(i)}) - \frac{i-1}{n}\right\}^+\right). \tag{3}$$

Then, we flag $\lfloor n d_n \rfloor$ observations among $X_1, \dots, X_n$ with the smallest depth values as cell-wise outliers.

## SM–5 Monte Carlo experiment

Results for all combinations of the model parameters explored in the Monte Carlo simulation are reported in this section.

In Figures 1, 2 and Figures 3, 4 the average LRT and average MSE versus different contamination values $k$ in cell-wise contamination are displayed, respectively.

Figures 5, 6 and Figures 7, 8 show the average LRT and average MSE versus different contamination values $k$, respectively, in the case of case-wise contamination.

Finally, Figure 9 reports the average LRT and average MSE versus the contamination value $k$ in the case of 20% case-wise contamination for increasing $n$, while the case of 2% cell-wise contamination is shown in Figure 10.

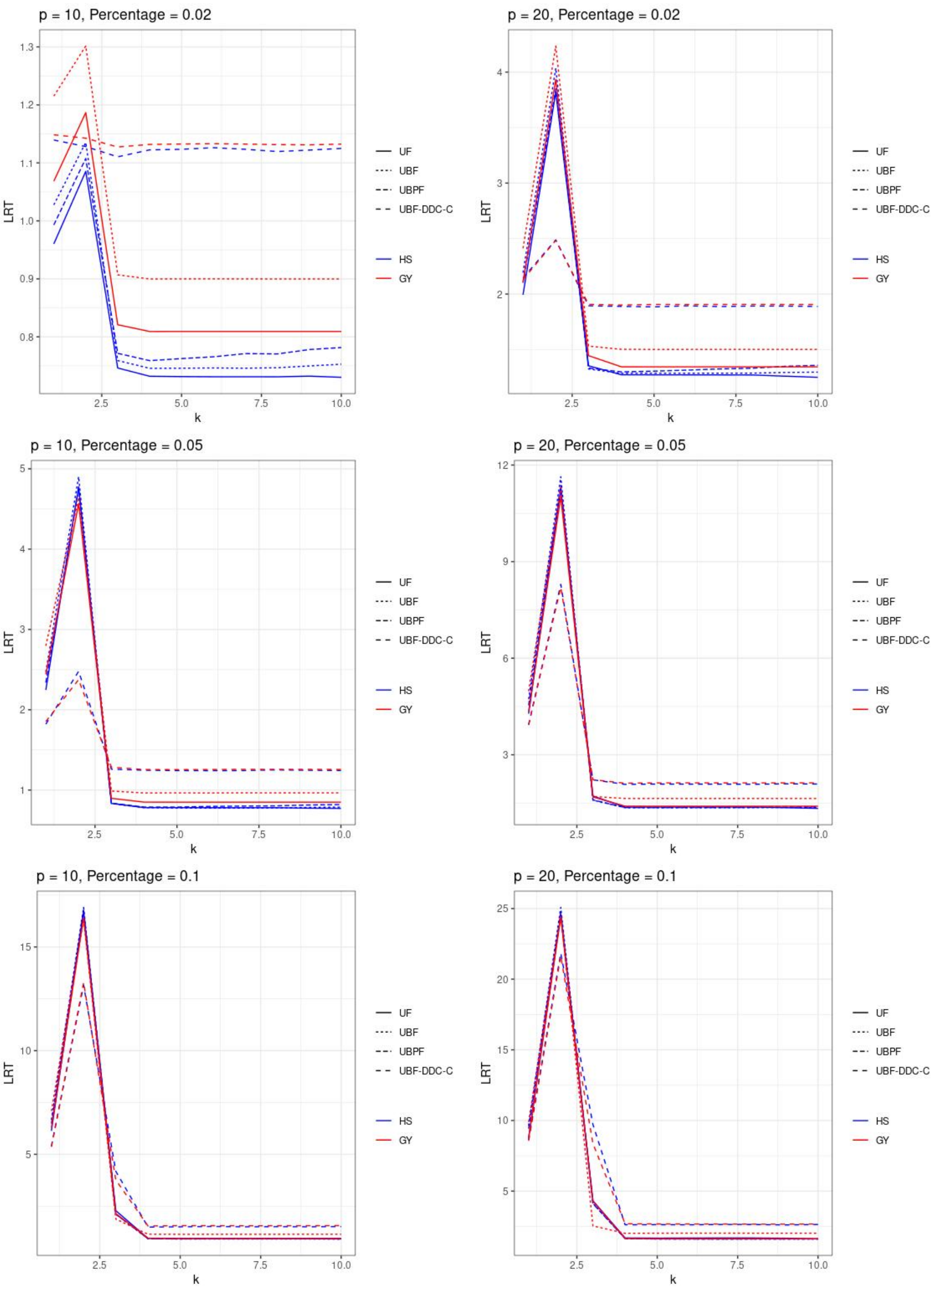


Figure 1: Average LRT versus the contamination value $k$ in cell-wise contamination, considering all combinations of contamination level $\epsilon$ and number of variables $p = 10, 20$.

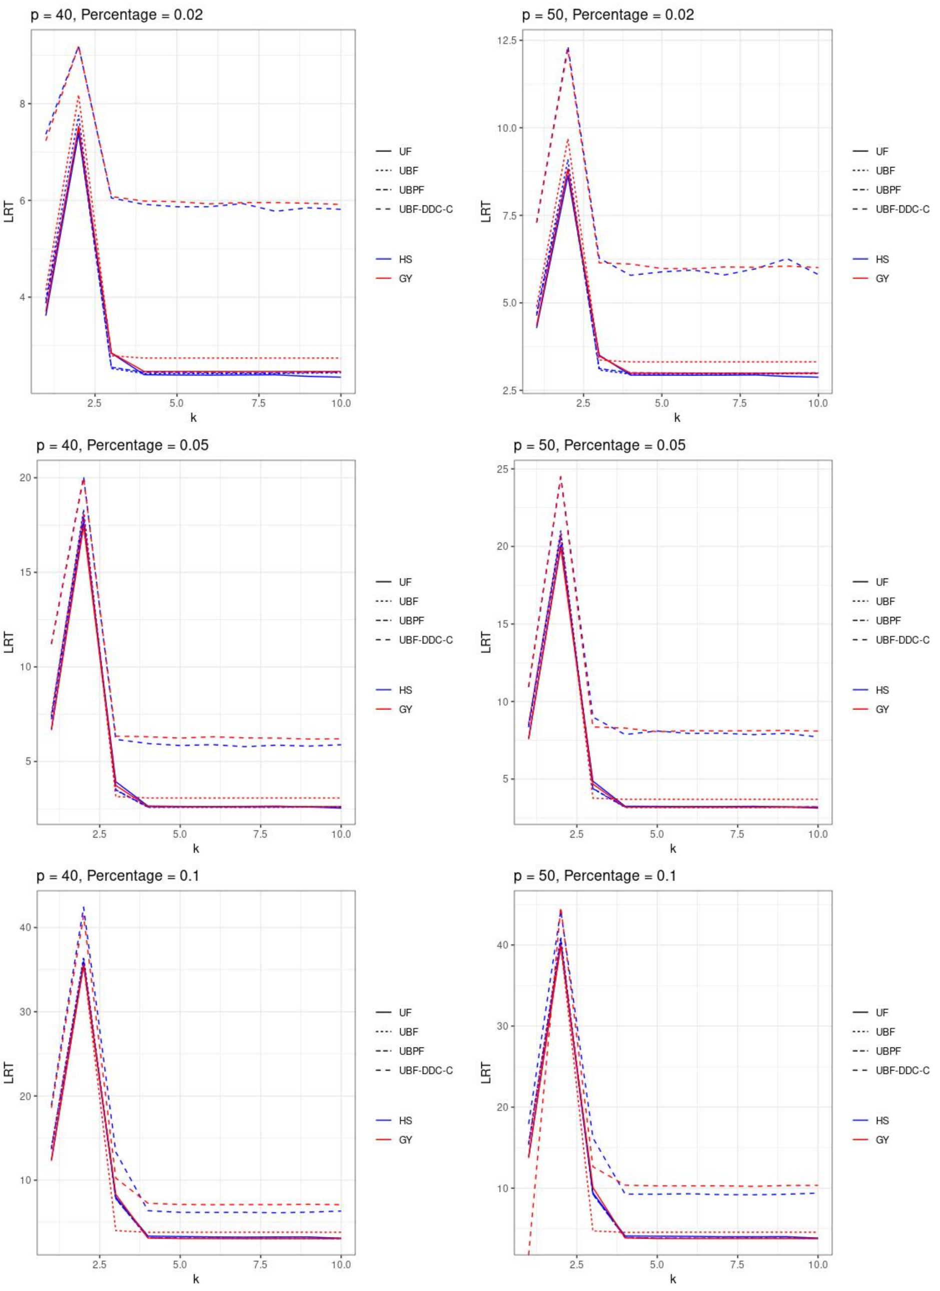


Figure 2: Average LRT versus the contamination value $k$ in cell-wise contamination, considering all combinations of contamination level $\epsilon$ and number of variables $p = 40, 50$.

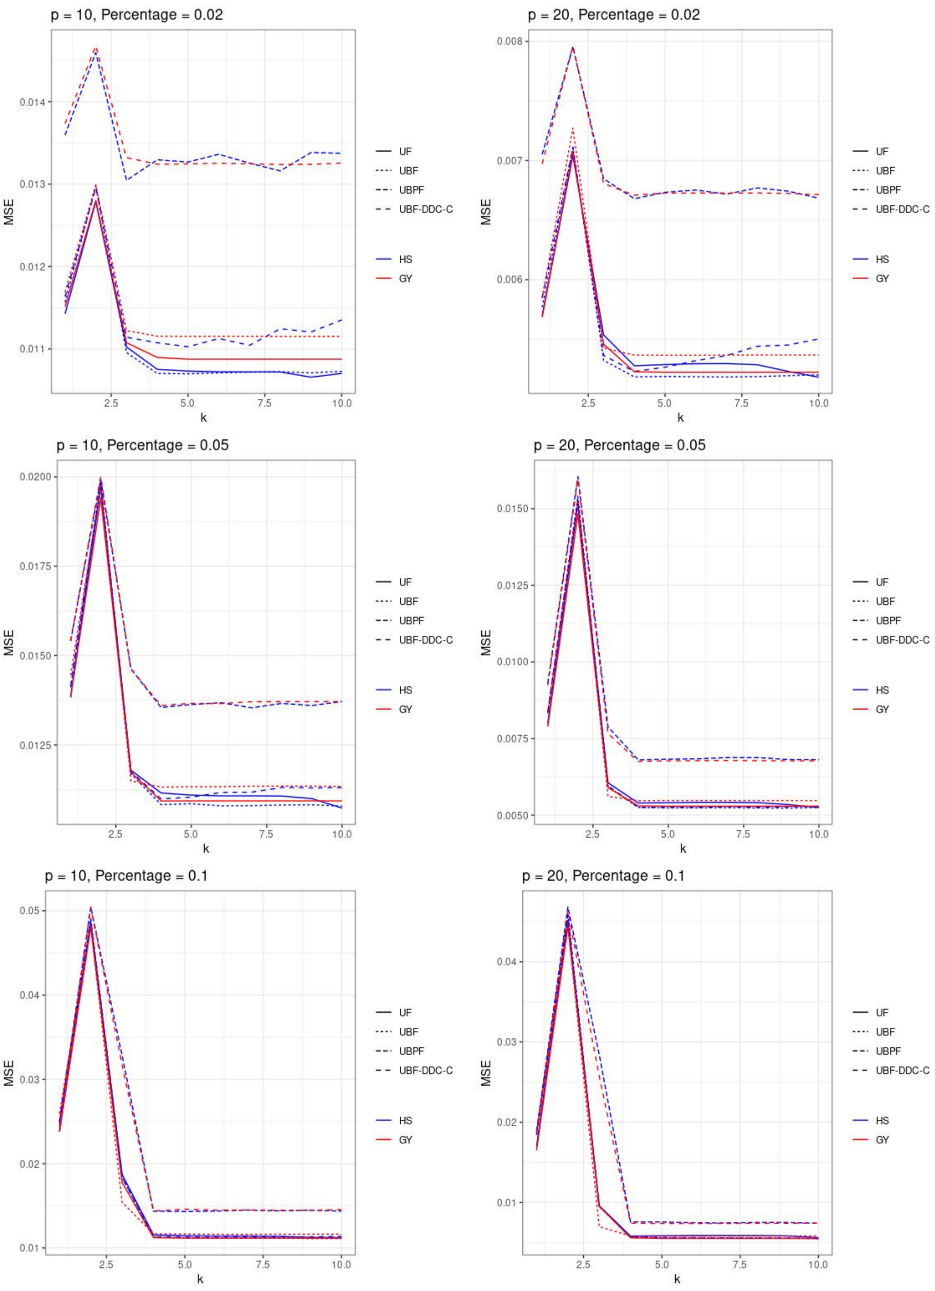


Figure 3: Average MSE versus the contamination value $k$ in cell-wise contamination, considering all combinations of contamination level $\epsilon$ and number of variables $p = 10, 20$.

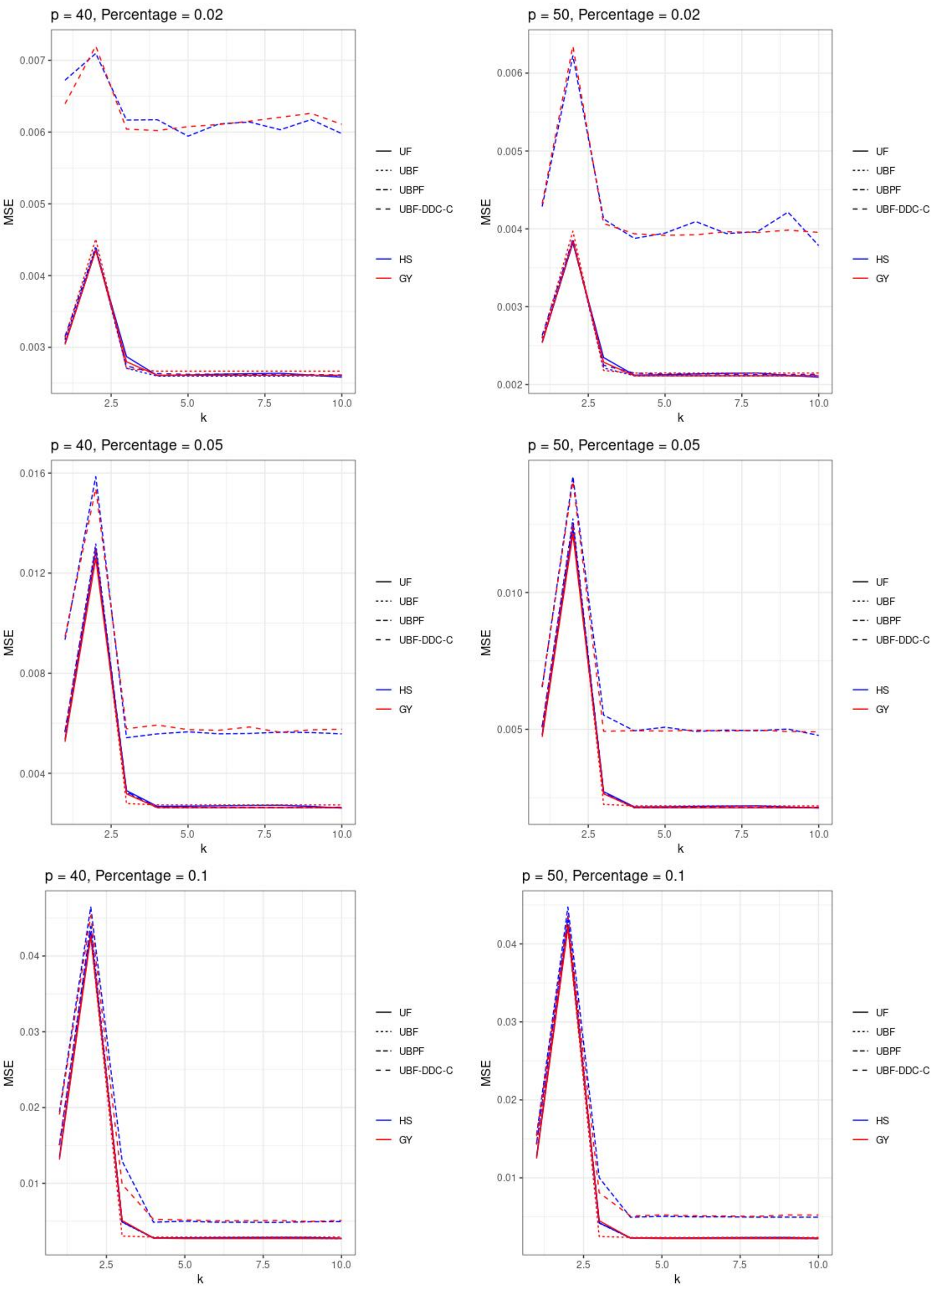


Figure 4: Average MSE versus the contamination value $k$ in cell-wise contamination, considering all combinations of contamination level $\epsilon$ and number of variables $p = 40, 50$.

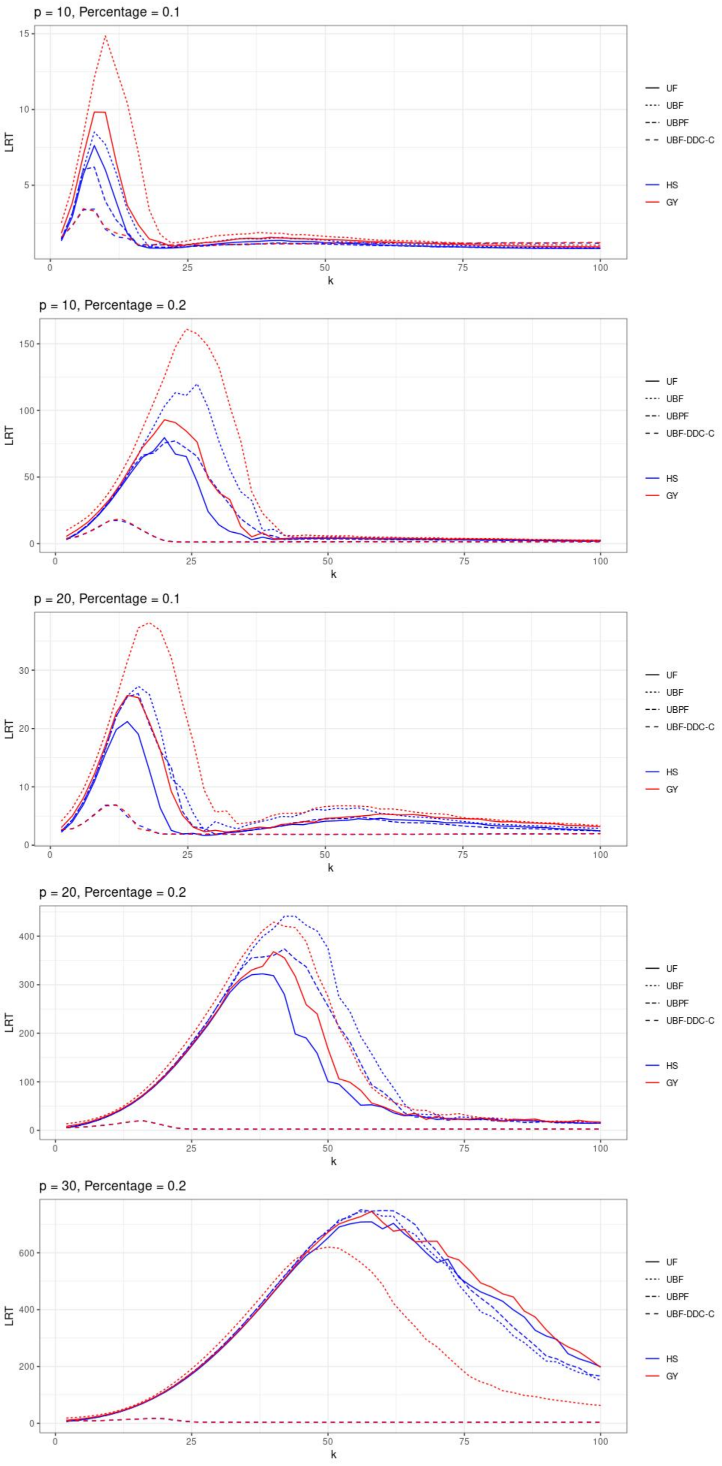


Figure 5: Average LRT versus the contamination value $k$ in case-wise contamination, considering all combinations of contamination level $\epsilon$ and number of variables $p = 10, 20, 30$.

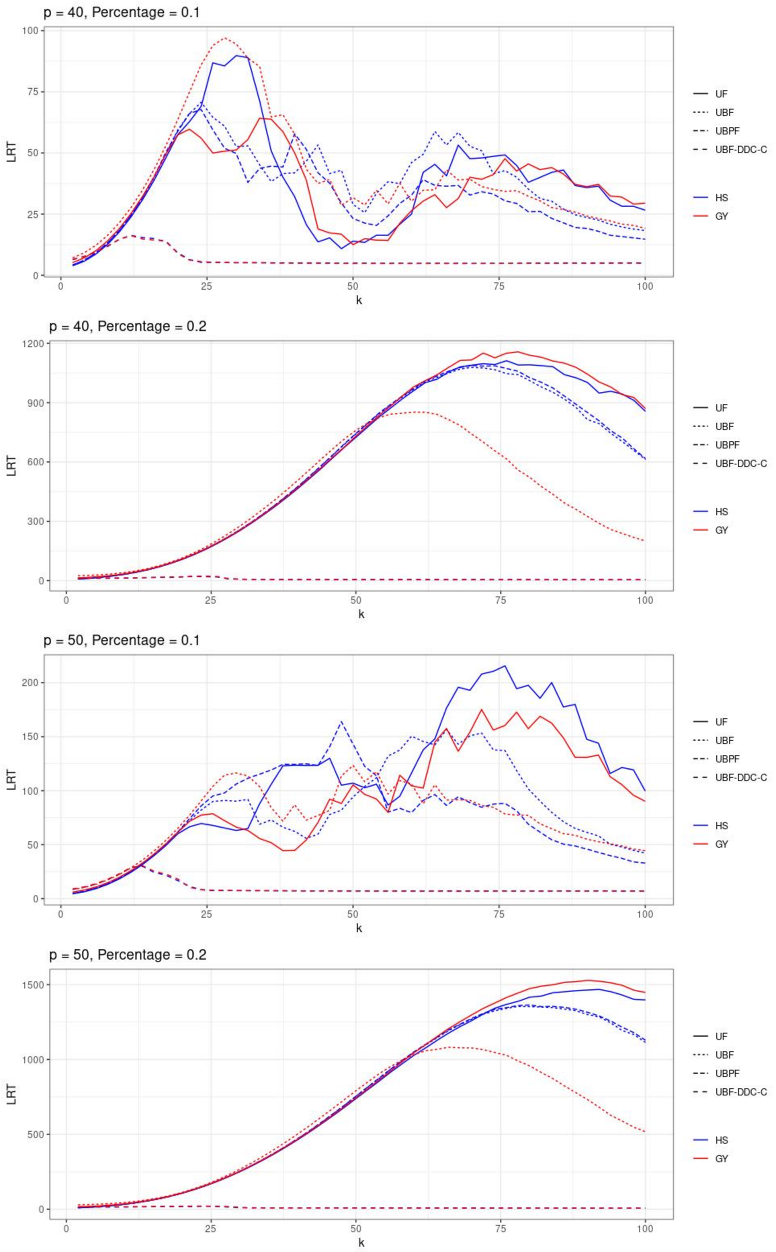


Figure 6: Average LRT versus the contamination value $k$ in case-wise contamination, considering all combinations of contamination level $\epsilon$ and number of variables $p = 40, 50$.

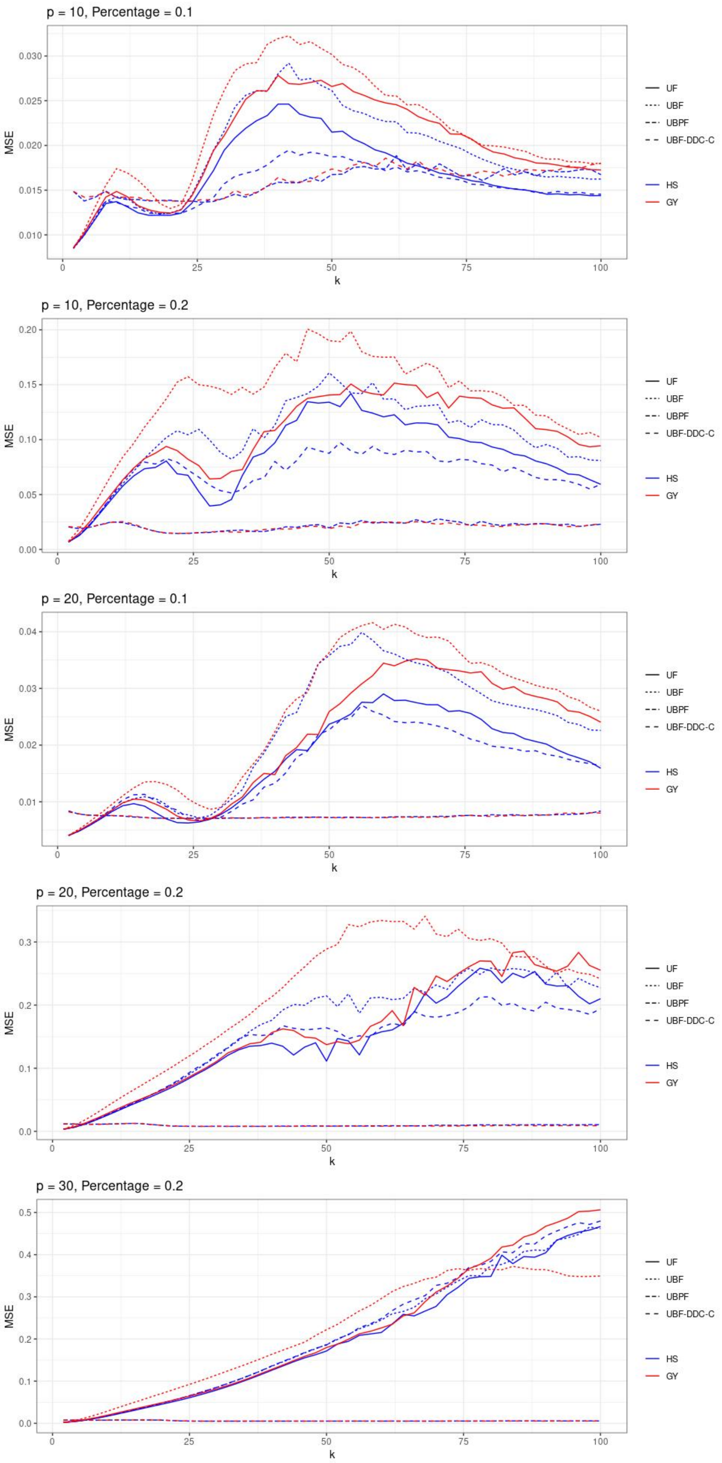


Figure 7: Average MSE versus the contamination value $k$ in case-wise contamination, considering all combinations of contamination level $\epsilon$ and number of variables $p = 10, 20, 30$.

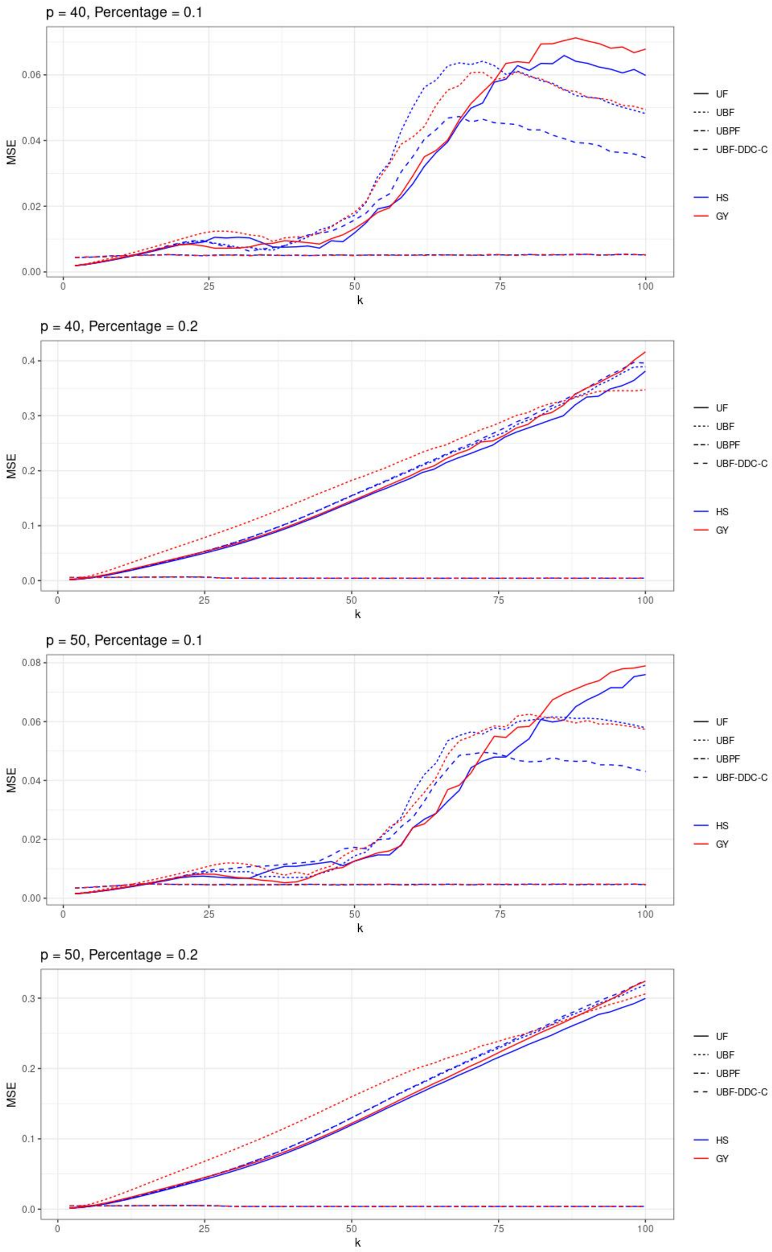


Figure 8: Average MSE versus the contamination value $k$ in case-wise contamination, considering all combinations of contamination level $\epsilon$ and number of variables $p = 40, 50$.

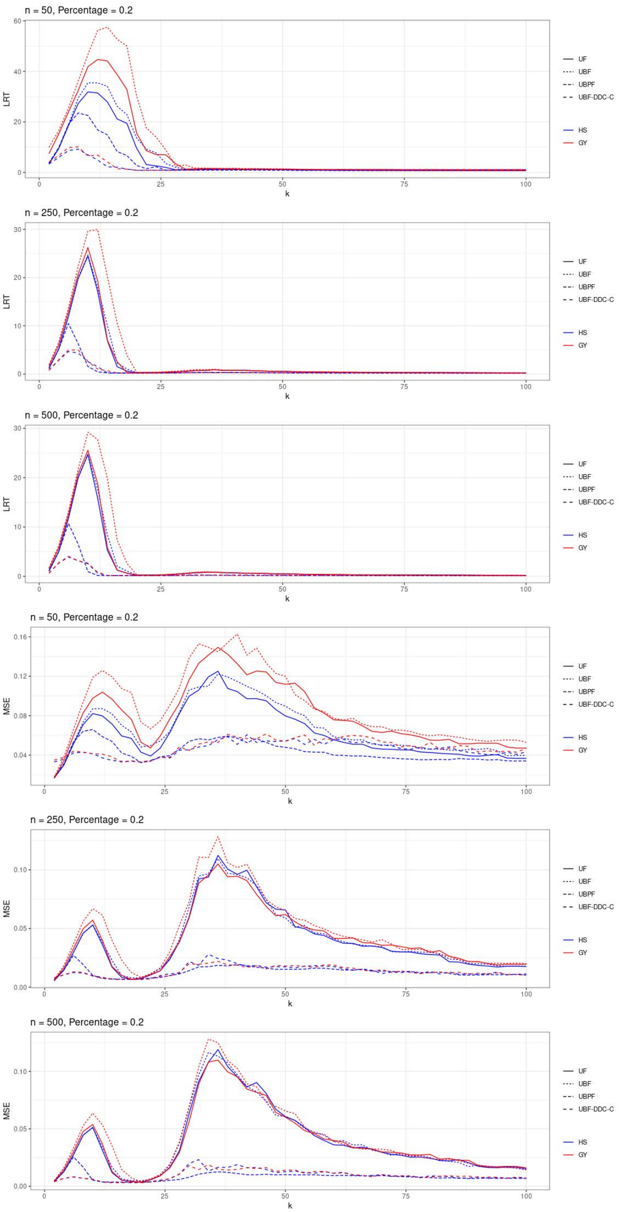


Figure 9: Average LRT (top) and average MSE (bottom) in 0.2 case-wise contamination level versus the contamination value $k$, for $p = 5$ and $n = 50, 250, 500$.

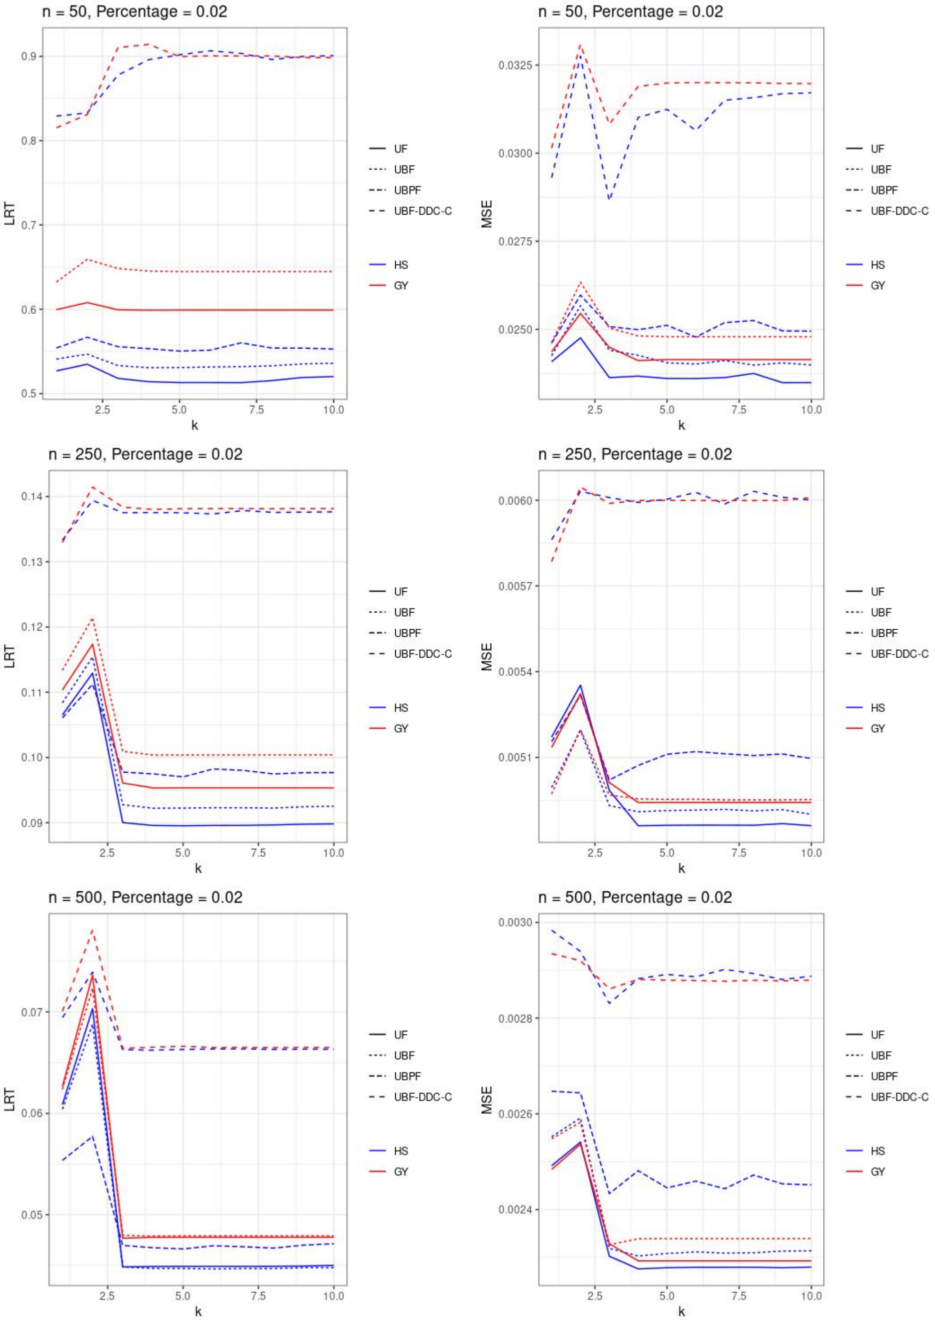


Figure 10: Average LRT (left) and average MSE (right) in 0.02 cell-wise contamination level versus the contamination value $k$, for $p = 5$ and $n = 50, 250, 500$.

# SM–6 R Code for the examples

## SM–6-1 Multivariate Skew-Normal distributions example

We consider a bivariate Skew-Normal distribution $\mathcal{SN}(\xi, \Omega, \alpha)$ with parameters $\xi = (0, 0)$, $\Omega = \boldsymbol{I}_2$ and $\alpha = (5, 5)$. This distribution will represents our chosen reference distribution.

```
> library(GSE)
> library(sn)
> library(ellipse)
> library(mvtnorm)
> library(ggplot2)
```

The expectation and the variance-covariance matrix used in the computation of the GY-filter are given by

```
> alpha <- c(5,5)
> e <- sqrt(2/pi)*(1+drop(alpha%*%alpha))^(-1/2)*alpha
> v <- diag(2) - e%*%t(e)
```

We define the function `f`, that computes the density of the reference distribution $F = \mathcal{SN}_2(\xi, \Omega, \alpha)$ with the parameter values chosen before, and the function `depth`, which approximated $d_{HS}((x, y), F)$, the population halfspace depth of a point $(x, y)$ with respect to $F$ by the sample halfspace depth of a large sample ($n = 100000$)

```
> f <- function(x, y) {
+   dmsn(x=c(x,y), xi=c(0,0), Omega=diag(2), alpha=alpha)
+ }
> set.seed(1234)
> dati <- rmsn(n=100000, xi=c(0,0), Omega=diag(2), alpha=alpha)
> depth <- function(x, y) {
+   depth.halfspace(x=c(x,y), data=dati, exact=FALSE, num.directions=100)
+ }
```

In order to plot their distributions, the density values of the reference distribution $F$ and the halfspace depth are computed for the points in a grid and stored in the matrices `zf` and `zdd` respectively.

```
> x <- seq(-2, 3, 0.2)
> zdd <- zf <- matrix(NA, nrow=length(x), ncol=length(x))
> for (i in 1:length(x)) {
+   for (j in 1:length(x)) {
```

```
+     zdd[i,j] <- depth(x[i], x[j])
+     zf[i,j] <- f(x[i], x[j])
+   }
+ }
```

We need two additional functions, `im` and `id`, which compute the fraction of outliers detected by the GY-filter and the HS-filter, respectively.

```
> im <- function(z) {
+   pmd <- mahalanobis(z, center=e, cov=v)
+   fn <- ecdf(pmd)
+   k <- qchisq(0.85, df=2)
+   dnm <- max((pchisq(pmd, df=2) - fn(pmd))[pmd > k])
+   dnm <- ifelse(dnm > 0, dnm, 0)
+   n0m <- floor(nrow(z)*dnm)
+   nrow(z)*dnm
+ }
> id <- function(z, ca) {
+   demp <- dteo <- depth.halfspace(z, z)
+   for (i in 1:nrow(z)) {
+     dteo[i] <- depth(z[i,1], z[i,2])
+   }
+   dnd <- max((demp-dteo)[dteo < ca])
+   dnd <- ifelse(dnd > 0, dnd, 0)
+   n0d <- floor(nrow(z)*dnd)
+   nrow(z)*dnd
+ }
```

Note that, in the function `id` we need to compute the value `ca` which identifies the boundary set $C^{\beta}(F)$. It is computed, in a numerical way, considering the population halfspace depth, using the following function.

```
> Calpha <- function(alpha=0.85, s=0.2) {
+   x <- seq(-2, 3, s)
+   g <- function(d) {
+     sum(zf[zdd > d])*s^2-alpha
+   }
+   uniroot(g, lower=0, upper=0.5)$root
+ }
> ca <- Calpha(0.85)
```

At this point, we simulate a sample of size $n = 100$ from $F$. The following code generates Fig. 5.

```
> set.seed(2345)
> z <- rmsn(n=100, xi=c(0,0), Omega=diag(2), alpha=alpha)
> plotdata2 <- data.frame(dati)
> plotdata3 <- data.frame(Z1=z[,1],Z2=z[,2])
> plotdata <- data.frame(x1=rep(x, each=length(x)),
+   x2 = rep(x,times=length(x)),
+   zdd = as.vector(zdd),zf = as.vector(zf))
> plotprova <- ggplot()+
+   theme_bw() +
+   geom_point(plotdata3,mapping=aes(x=Z1,y=Z2),col="blue",shape=3) +
+   stat_contour(plotdata,mapping=aes(x=x1, y=x2, z=zf),col="black",lty=3) +
+   stat_contour(plotdata,mapping=aes(x=x1,y=x2,z=zdd),
+     breaks = c(ca,0.05, seq(0.1,0.9,0.1)),colour = "red",lty="dashed") +
+   xlab(expression(x[1])) +
+   ylab(expression(x[2]))
```

We are going to add artificially 20 outliers which lie, with high probability, inside the boundary set given by the Mahalanobis distance but outside the boundary set computed using the halfspace depth. The following code is the implementation of the iterative procedure used.

```
> # Generate outlying observations.
> k <- 20
> set.seed(2345)
> plotdata4 <- data.frame(out = rmvnorm(20,mean = c(-0.2,-0.25),
+   sigma = 0.01*diag(2)))
> colnames(plotdata4) <- c("Z1","Z2")
> # Iterations:
> zd1 <- zm1 <- rep(0,k)
> for (i in 1:k) {
+   # Add an outlier.
+   z <- rbind(z,as.numeric(plotdata4[i,]))
+
+   # Compute number of flagged cells.
+   zd1[i] <- floor(id(z, ca))
+   zm1[i] <- floor(im(z))
+
+   # Compute theoretical depth to identify the outlying cells for
+   # the depth-filter.
+   d.teo <- rep(0,nrow(z))
+   for (j in 1:nrow(z)) {
+     d.teo[j] <- depth(z[j,1], z[j,2])
```

```
+   }
+   dd <- sort(d.teo)[zd1[i]]
+   outd <- which(d.teo <= dd)
+
+   # Compute the Mahalanobis distance to identify the outlying cells
+   # for the GY-filter.
+   pmd <- mahalanobis(z, center=e, cov=v)
+   ddm <- sort(pmd,decreasing = TRUE)[zm1[i]]
+   outm <- which(pmd >= ddm)
+
+   # Create a plot
+   plotdata5 <- rbind(plotdata3,plotdata4[1:i,])
+   plotprova <- ggplot()+
+     theme_bw() +
+     # Sampled observations
+     geom_point(plotdata3,mapping=aes(x=Z1,y=Z2),col="blue",shape=3) +
+     # Depth contours
+     stat_contour(plotdata,mapping=aes(x=x1,y=x2,z=zdd),
+       breaks = c(0.05, seq(0.1,0.9,0.1)),colour = "red",lty="dashed") +
+     stat_contour(plotdata,mapping=aes(x=x1,y=x2,z=zdd),
+       breaks = c(ca),colour = "red") +
+     xlab(expression(x[1])) +
+     ylab(expression(x[2])) +
+     # Boundary set of GY-filter
+     stat_ellipse(plotdata2,mapping=aes(x=X1,y=X2),col="green") +
+     # Added outliers
+     geom_point(plotdata4[1:i,],mapping=aes(x=Z1,y=Z2),col="black",shape=1) +
+     # Observations flagged by the depth-filter
+     geom_point(plotdata5[outd,],mapping=aes(x=Z1,y=Z2),col="red",shape=4) +
+     # Observations flagged by the GY-filter
+     geom_point(plotdata5[outm,],mapping=aes(x=Z1,y=Z2),col="green",shape=2)
+
+   # Save the generated plot
+   ggsave(plotprova, filename = paste0("sn-ggplot-", i, ".pdf", sep=""),
+          device = "pdf",height = 5,width = 7)
+ }
```

The plot saved at the end of the last iteration correspond to Fig. 6. Moreover, the vectors `zd1` and `zm1` store the number of flagged observations by the depth-filter and the GY-filter, respectively, in each iteration, and have been reported in Table 5. Finally, the following code is similar to the previous one

and it has been used for the second experiment, where the added outlying observations lie, with high probability, outside the boundary set given by the Mahalanobis distance.

```
> set.seed(2345)
> z <- rmsn(n=100, xi=c(0,0), Omega=diag(2), alpha=alpha)
> # Generate  outlying observations.
> k <- 20
> x <- seq(-2, 3, 0.2)
> set.seed(1234)
> plotdata4 <- data.frame(out = rmvnorm(20,mean = c(-0.5,-0.6),
+                                       sigma = 0.01*diag(2)))
> colnames(plotdata4) <- c("Z1","Z2")
> # Iterations:
> zd2 <- zm2 <- rep(0,k)
> for (i in 1:k) {
+   # Add new observation and compute the number of flagged points
+   z <- rbind(z,as.numeric(plotdata4[i,]))
+   zd2[i] <- floor(id(z, ca))
+   zm2[i] <- floor(im(z))
+   # Identify flagged observations
+   d.teo <- rep(0,nrow(z))
+   for (j in 1:nrow(z)) {
+     d.teo[j] <- depth(z[j,1], z[j,2])
+   }
+   dd <- sort(d.teo)[zd2[i]]
+   outd <- which(d.teo <= dd)
+
+   pmd <- mahalanobis(z, center=e, cov=v)
+   ddm <- sort(pmd,decreasing = TRUE)[zm2[i]]
+   outm <- which(pmd >= ddm)
+
+   # Generate and save the plot
+   plotdata5 <- rbind(plotdata3,plotdata4[1:i,])
+   plotprova <- ggplot()+
+     theme_bw() +
+     geom_point(plotdata3,mapping=aes(x=Z1,y=Z2),col="blue",shape=3) +
+     stat_contour(plotdata,mapping=aes(x=x1,y=x2,z=zdd),
+       breaks = c(0.05, seq(0.1,0.9,0.1)),colour = "red",lty="dashed") +
+     stat_contour(plotdata,mapping=aes(x=x1,y=x2,z=zdd),
+       breaks = c(ca),colour = "red") +
```

```
+      xlab(expression(x[1])) +
+      ylab(expression(x[2])) +
+      stat_ellipse(plotdata2,mapping=aes(x=X1,y=X2),col="green") +
+      geom_point(plotdata4[1:i,],mapping=aes(x=Z1,y=Z2),col="black",shape=1) +
+      geom_point(plotdata5[outd,],mapping=aes(x=Z1,y=Z2),col="red",shape=4) +
+      geom_point(plotdata5[outm,],mapping=aes(x=Z1,y=Z2),col="green",shape=2)
+
+    ggsave(plotprova,
+           filename = paste0("sn-ggplot-outside-", i, ".pdf", sep=""),
+           device = "pdf",height = 5,width = 7)
+ }
```

Plots saved in the $10^{th}$ and in the final iteration are displayed in Fig. 7 and, as before, the information in the vectors zd2 and zm2 is reported in Table 6.

## SM–6-2 Small-cap Stock Returns

After loading the data set, included in the R package GSEdepth, we select the observations corresponding to the period from 01/01/2008 to 12/28/2010 for the variables representing the 20 stock returns, accordingly to Leung et al. [2017].

```
> library(GSE)
> library(GSEdepth)
> library(lattice)
> data("small_cap")
> str(small_cap)
> colnames(small_cap)
> cap <- small_cap[574:730,2:21]
> dim(cap)
```

A data point is considered outlier if it lies 3 standard deviations away from the median. The following code has been used to count the number of cellwise outlier detected according to this rule and the number of rows that contain at least one contaminated cell. The detected cells are showed in green in Fig. 8.

```
> count <-0
> rows <- c()
> outliers <- list()
> outlier_varible <- matrix(0,nrow=nrow(cap), ncol=ncol(cap))
> for(i in 1:ncol(cap)){
```

```
+   var <- cap[,i]
+   med_var <- median(var)
+   mad_var <- mad(var)
+   out <- which(abs(var - med_var) >  3*mad_var )
+   outliers[[i]] <- out
+   rows <- unique(c(rows,out))
+   count <- count + length(out)
+   outlier_varible[out,i] <- 1
+ }
```

After this preliminary analysis, we apply the GY-filters and the HS-filters.

```
> est_mle <- mlest(cap)
> est_uf <- TSGSd(cap, filter = "UF")
> est_ubf <- TSGSd(cap, filter = "UBF")
> est_ub_ddc <- TSGSd(cap, filter = "UBF-DDC",
+                     method = "rocke", init = "emve_c")
> est_dep_uf <- TSGSd(cap, filter = "depth-UF")
> est_dep_ubf <- TSGSd(cap, filter = "depth-UBF")
> est_dep_ubpf <- TSGSd(cap, filter = "depth-UBPF")
> est_ubp_ddc <- TSGSd(cap, filter = "depth-UBPF",
+                      method = "rocke",init = "emve_c")
```

The obtained location and scale estimates are used to compute the Mahalanobis distances displayed in Fig. 9. The following code gives an example.

```
> # Mahalanobis distances
> pmd_dep_est_ubf <- mahalanobis(cap, est_dep_ubf@mu, est_dep_ubf@S)
> # Modification for a better visualization
> pmd_dep_est_ubf[which(pmd_dep_est_ubf > 150)] <- 150
> # Plot
> plot(as.Date(small_cap$DATE[574:730],"%m/%d/%Y"), pmd_dep_est_ubf,
+      col=c("black", "green")[fatt], pch = 19, main= "depth-UBF",
+      ylab= "Squared Mahalanobis Distance", xlab = "Weeks")
> abline(h = qchisq(0.9999, 20), col = "red")
> # Number of observations with a large Mahalanobis distance
> length(which(pmd_dep_est_ubf > qchisq(0.9999, 20)))
> # Number of observations with a large Mahalanobis distance
> # previously identified as outliers.
> length(which(pmd_dep_est_ubf[which(fatt==1)] > qchisq(0.9999, 20)))
```

# References

D. Gervini and V.J. Yohai. A class of robust and fully efficient regression estimators. *The Annals of Statistics*, 30(2):583–616, 2002.

R.Y. Liu. On a notion of data depth based on random simplices. *The Annals of Statistics*, 18(1):405–414, 1990.

R.J. Serfling. Multivariate symmetry and asymmetry. *Encyclopedia of statistical sciences*, pages 5338–5345, 2006.

Y. Zuo and R. Serfling. General notions of statistical depth function. *The Annals of Statistics*, 28(2):461–482, 2000.
